# Supplementary material for: Direct observation of ultrafast long-range charge separation at polymer:fullerene heterojunctions
Source: arXiv:1310.8331 ancillary file (2013-10-30)
Supplement: Supplementary file 1 [file Provencher_Supplementary_Information.pdf]

**Supplementary Information for**

# Direct observation of ultrafast long-range charge separation at polymer:fullerene heterojunctions

Françoise Provencher, Nicolas Bérubé, Anthony Parker, Gregory M. Greetham, Michael Towrie, Christoph Hellmann, Michel Côté, Natalie Stingelin, Carlos Silva and Sophia C. Hayes

## Ultrafast polaron signature

We see in the blend FSRS spectra at room temperature that the 1350 $cm^{-1}$ band, characteristic of positive polaron, appears as early as 100 fs.

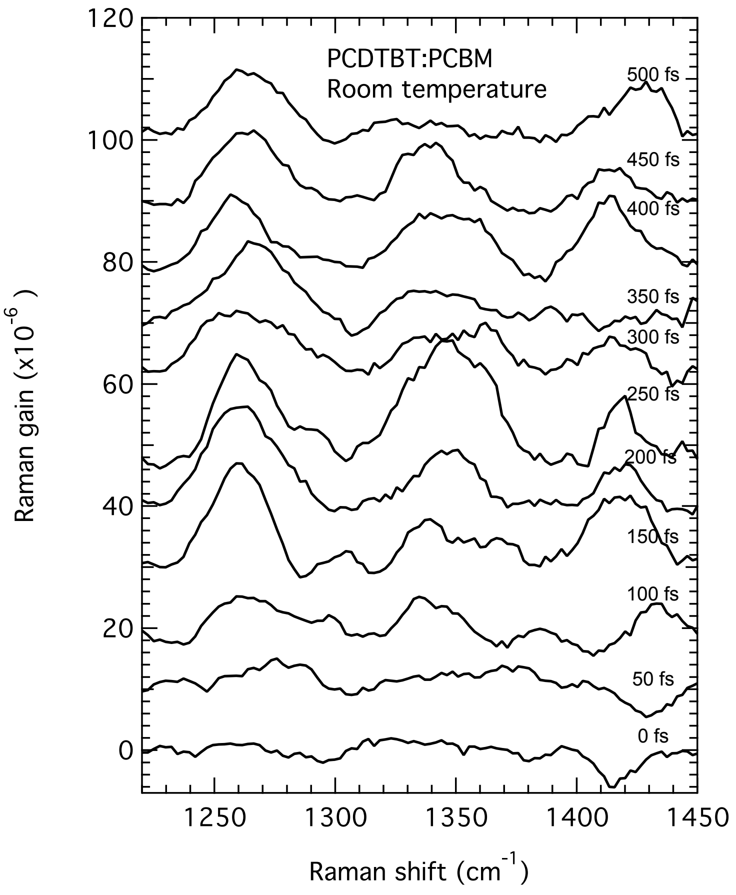


**Figure S1 :** Transient stimulated resonance Raman spectra of PCDTBT:PCBM film at early times.

## Calculated spectra

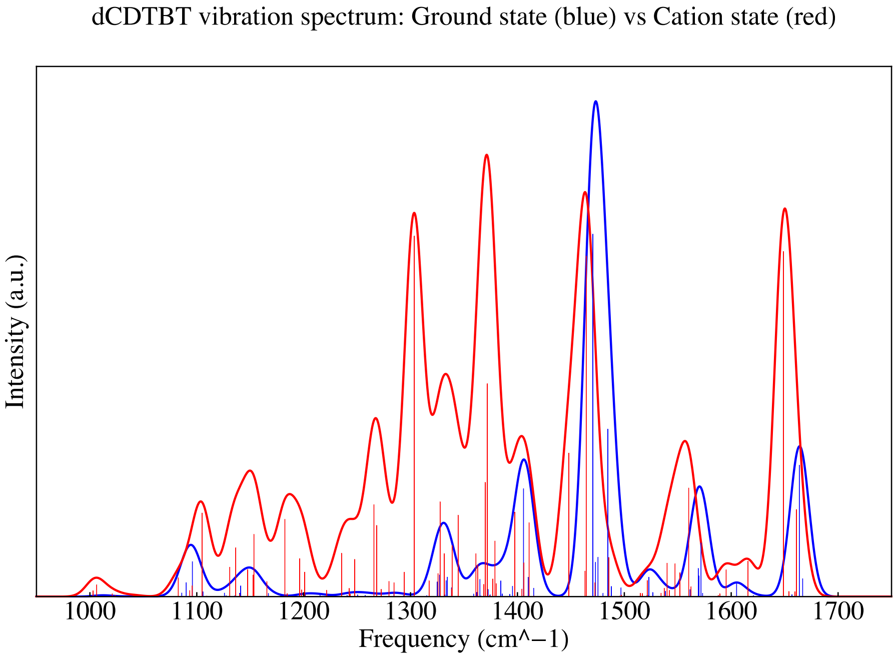


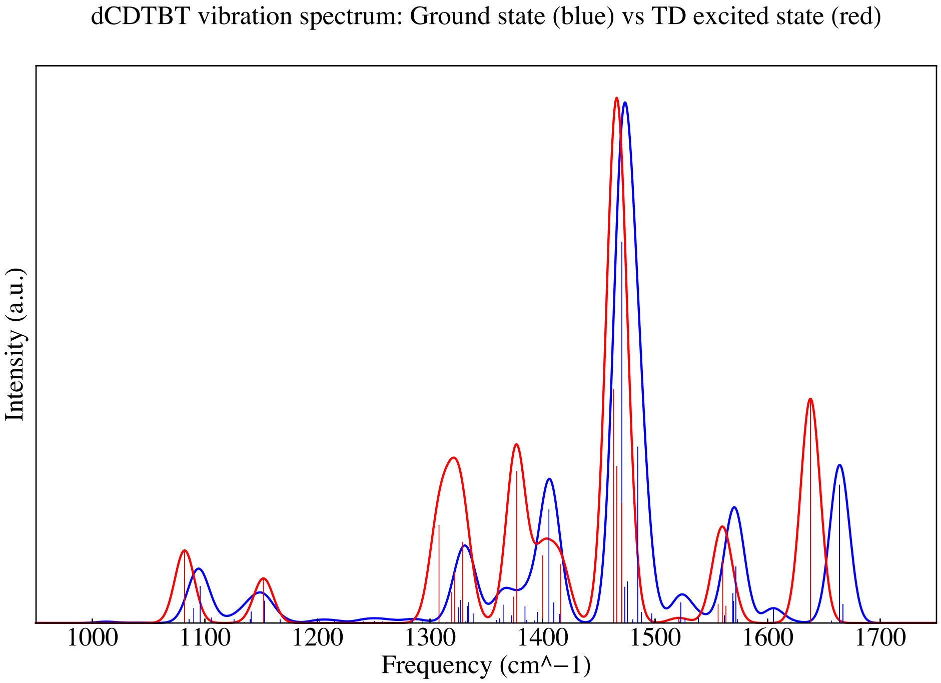


**Figure S2** : Calculated spectra for neat PCDTBT dimers in the ground state (blue) and either the cation (red, top) or the exciton (red, bottom).

## Spontaneous Raman spectra

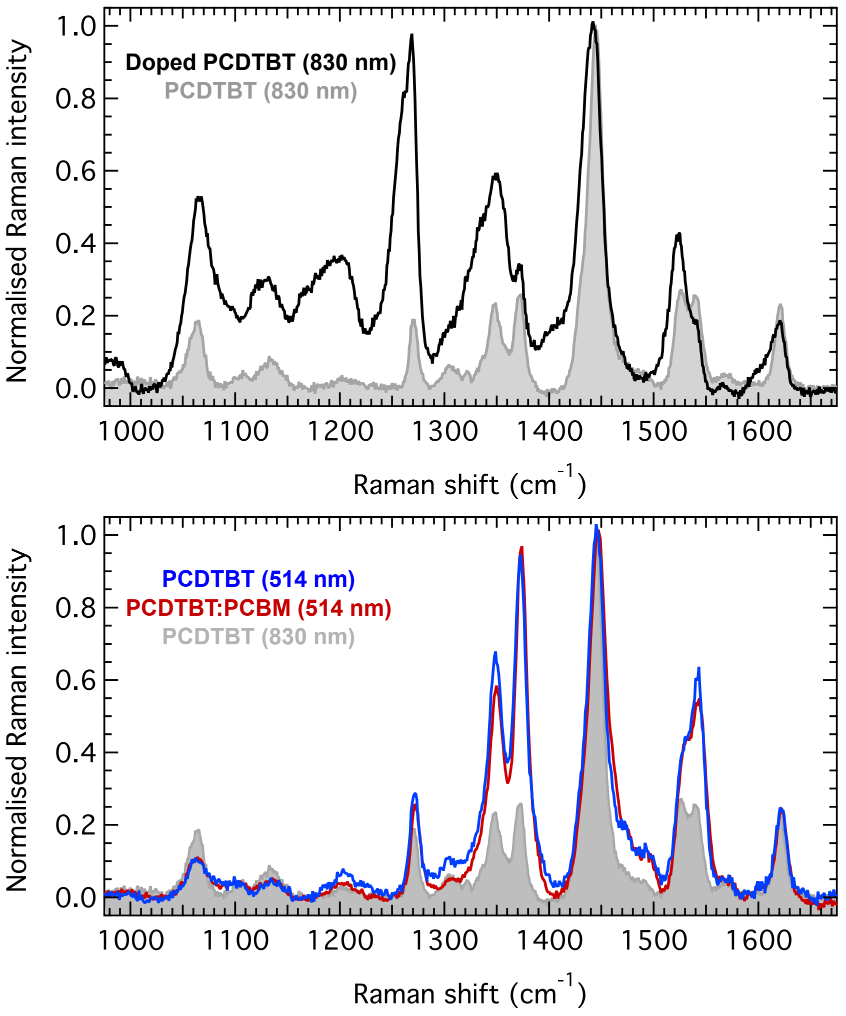


**Figure S3** : Steady-state spontaneous Raman spectra of doped PCDTBT (top) and neat PCDTBT and PCDTBT:PCBM (bottom) films under resonant conditions, compared to non-resonant Raman spectrum (gray area).

**Normalised FSRS spectra**

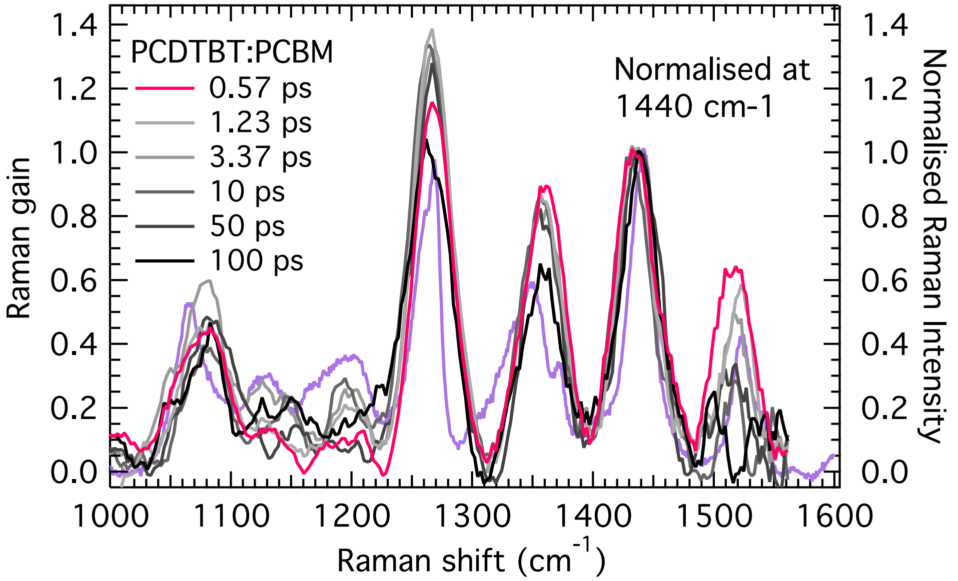


**Figure S4** : FSRS spectra of PCDTBT:PCBM film, normalised at 1440 $cm^{-1}$ to show relative peak intensities evolution compared to steady-state spontaneous resonance Raman of doped PCDTBT (violet line). The spectral region between 1100 and 1230 $cm^{-1}$ suffers from difficult background subtraction, which makes the evolution of the 1200 $cm^{-1}$ band dynamics difficult to follow.

After 50 ps, we observe a decay of the 1261 and 1364 $cm^{-1}$ bands which further emulate the relative intensities in the cationic spectrum.

## Characterisation of polymer thin films microstructure

In order to characterise the microstructure and molecular arrangement in this material system, X-ray diffraction experiments were performed. The corresponding powder diffractograms of drop-cast neat PCDTBT, neat PCBM and its blend film (1 part polymer : 4 parts fullerene by weight) are illustrated in figure S5. In agreement with the results of previous reports, the neat PCDTBT sample shows broad diffractions at angles with maximum intensities around 4° and 22°, suggesting crystallographic low conformational order.[1,2]

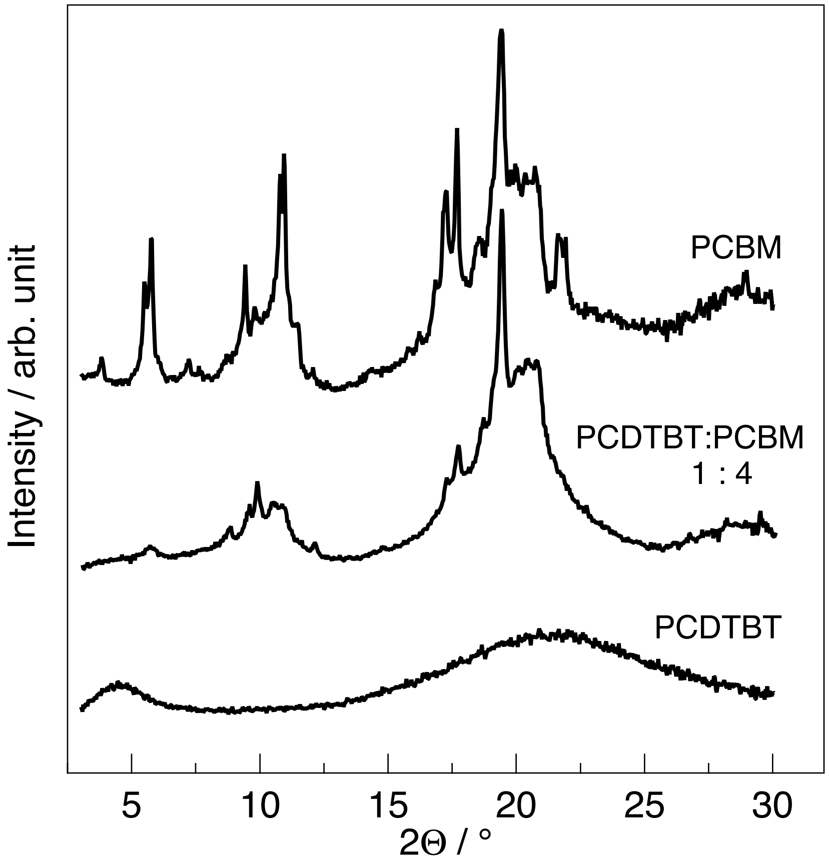


**Figure S5 :** X-ray diffractograms of drop casted neat PCDTBT, neat PCBM and its blend (1 part polymer : 4 parts fullerene)

After blending the PCDTBT with the fullerene derivative, the broad diffraction at 4°, related to the neat polymer, can not be distinguished in the blend system with 80 wt% PCBM anymore. The presence of the fullerene derivative in excess obviously leads to further crystallographic disorder of the polymer chains. Crystalline domains of PCBM remain however within the blend when drop cast from DCB at 100°C. Main diffractions of these PCBM domains were recorded at angles around 10, 17, 19° and reveal the molecular packing in complex crystallographic unit cells[3,4] comparable to the diffractions of our neat PCBM sample.

In order to gain further structural information of the neat polymer, the neat fullerene derivative and the blend system, we concentrate our efforts on combining optical and thermal characterisation techniques. Optical microscopic images of the films were taken at selected temperatures and compared to thermal transitions recorded from differential scanning calorimetry (DSC) experiments (see figure S6).

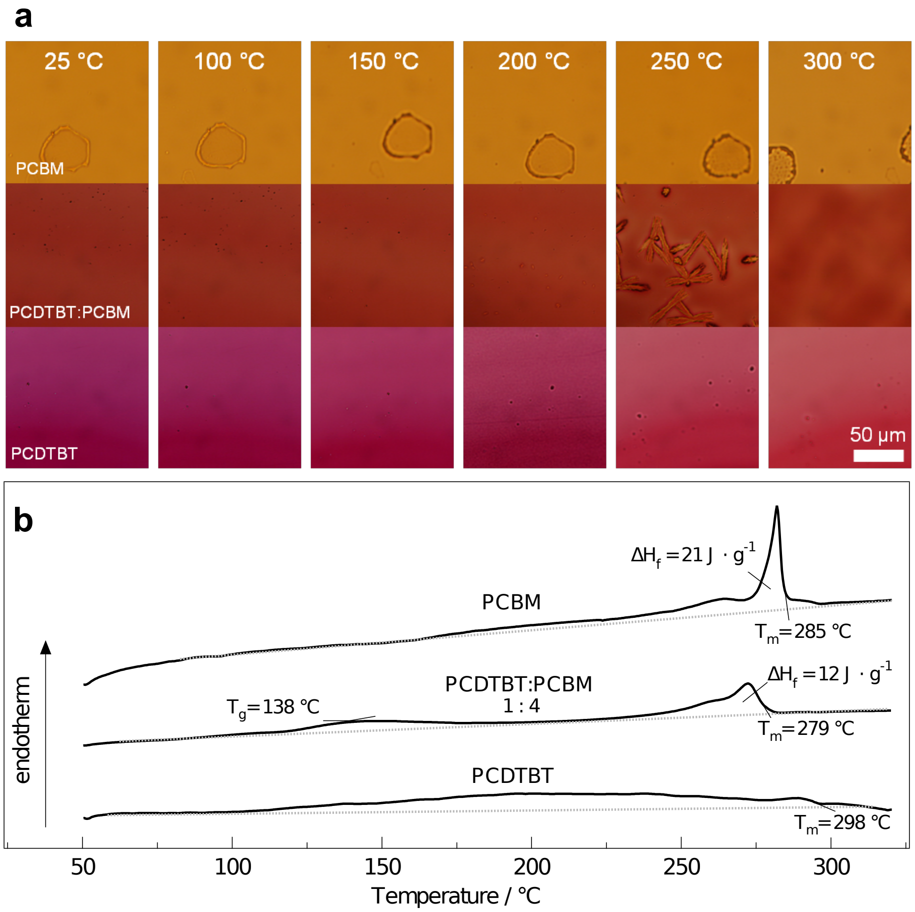


**Figure S6 :** (a) Optical micrographs of PCDTBT, PCBM and its blend films at selected temperatures and (b) corresponding differential scanning calorimetric thermograms.

Following our film formation protocol smooth films are formed of the neat materials and the blend. During heating from 25 up to 300 °C the featureless films of the neat PCDTBT and the PCBM remain essentially unchanged. However, the transition of colour between 25 and 300 °C from dark purple to pink in the neat PCDTBT system indicate less conformational order and aggregation in the isotropic melt compared to the solid state of the polymer. For the blend, homogeneous and featureless films are formed which appear unchanged using our optical microscopic technique until a temperature of approximately 200 °C is reached. At this temperature the formation of needle like PCBM crystallites could be observed which has been also reported for diverse

polymer:fullerene systems during thermal treatment.[5-7] During further heating these PCBM features become clearly distinguishable in our experiment at a temperature of 250 °C. If the temperature is further increased to 300 °C both materials reach their liquid state. Investigations revealing kinetic information about the nucleation and growth rate of PCBM crystallites would give further insight into the mixing/demixing characteristics of this system but this is beyond the scope of this work.

The thermograms of the neat PCDTBT and neat PCBM films, drop-cast from solutions in DCB at 100°C shown here, are in accordance with reported thermal induced conformational changes found for these systems.[1] Films of neat PCDTBT indicate an onset of thermal induced chain movements in disordered fraction above approximately 100°C, which is supported by the reported glass transition temperature ($T_g$) of 130°C.[1] Around 298°C a weakly pronounced endotherm indicates the melting of more ordered regions of the polymer chains. The thermogram of neat PCBM films shows a pronounced melting peak of crystalline domains with an end of melting at approximately 285°C. Please note that the main melting endotherm shows additional melting features at the on and off set of the main peak which we relate to different conformational arrangements of the fullerene derivative formed under our solidification /crystallisation conditions.

The elucidation of the complex morphology in polymer : fullerene systems has been subject of intense investigations. Pure polymer (amorphous and crystalline domains), pure fullerene (amorphous and crystalline domains) and intermixed phases (amorphous domains) have been reported, e. g. in systems containing poly 3-hexylthiophene (P3HT) and multiple $C_{60}$ fullerene derivatives.[5-7] Our efforts in this study concentrate on the formation of possible pure amorphous, pure crystalline and intermixed domains of the fullerene component in the disordered polymer regions. In addition to the results of the X-ray diffraction experiments, a defined melting transition of PCDTBT can not be distinguished from the thermogram of the blend system, which also indicates a less ordered polymer arrangement if blended with PCBM. Please note, that in this experiment no exothermic transition due to crystallisation of the fullerene could be recorded.

Furthermore, our DSC data reveal that the fullerene derivative can mix with the selected polymer system. This idea is supported by the observed melting point depression of approximately 6 °C from 285 down to 279 °C for the residual crystalline fullerene component in the blend system. Additionally, the difference of the enthalpy of fusion ($\Delta H_f$) of the fullerene derivative is reduced from approximately 21 down to around 12 $J \cdot g^{-1}$ which one would expect in a partly miscible system. Please note that a weak endothermic transition at around 138°C was recorded which could be related to the glass transition temperature of this blend system. Further investigations are ongoing to clarify this point but this out of the scope of this manuscript.

## Baseline subtraction example

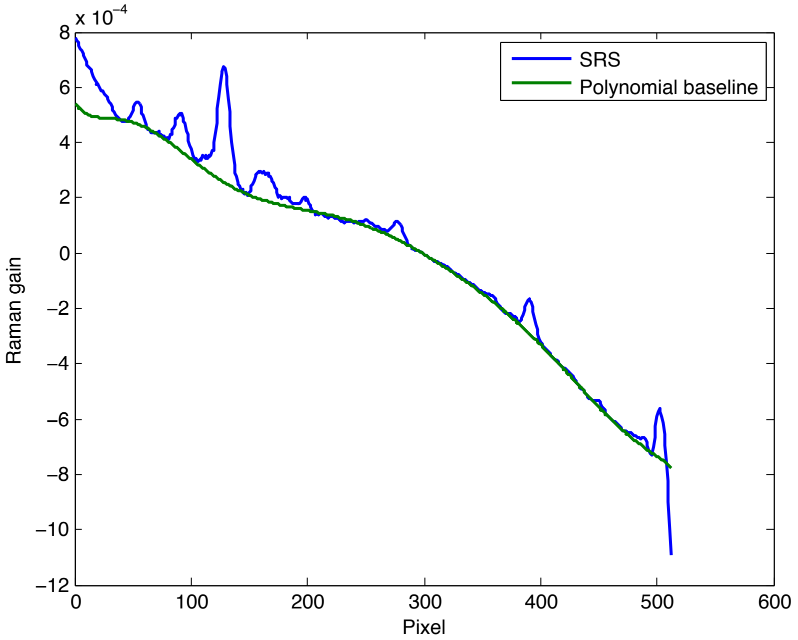


**Figure S7 :** Example of polynomial baseline subtraction on smoothed FSRS spectrum.

## FSRS spectra of PCDTBT and PCDTBT:PCBM at all recorded times

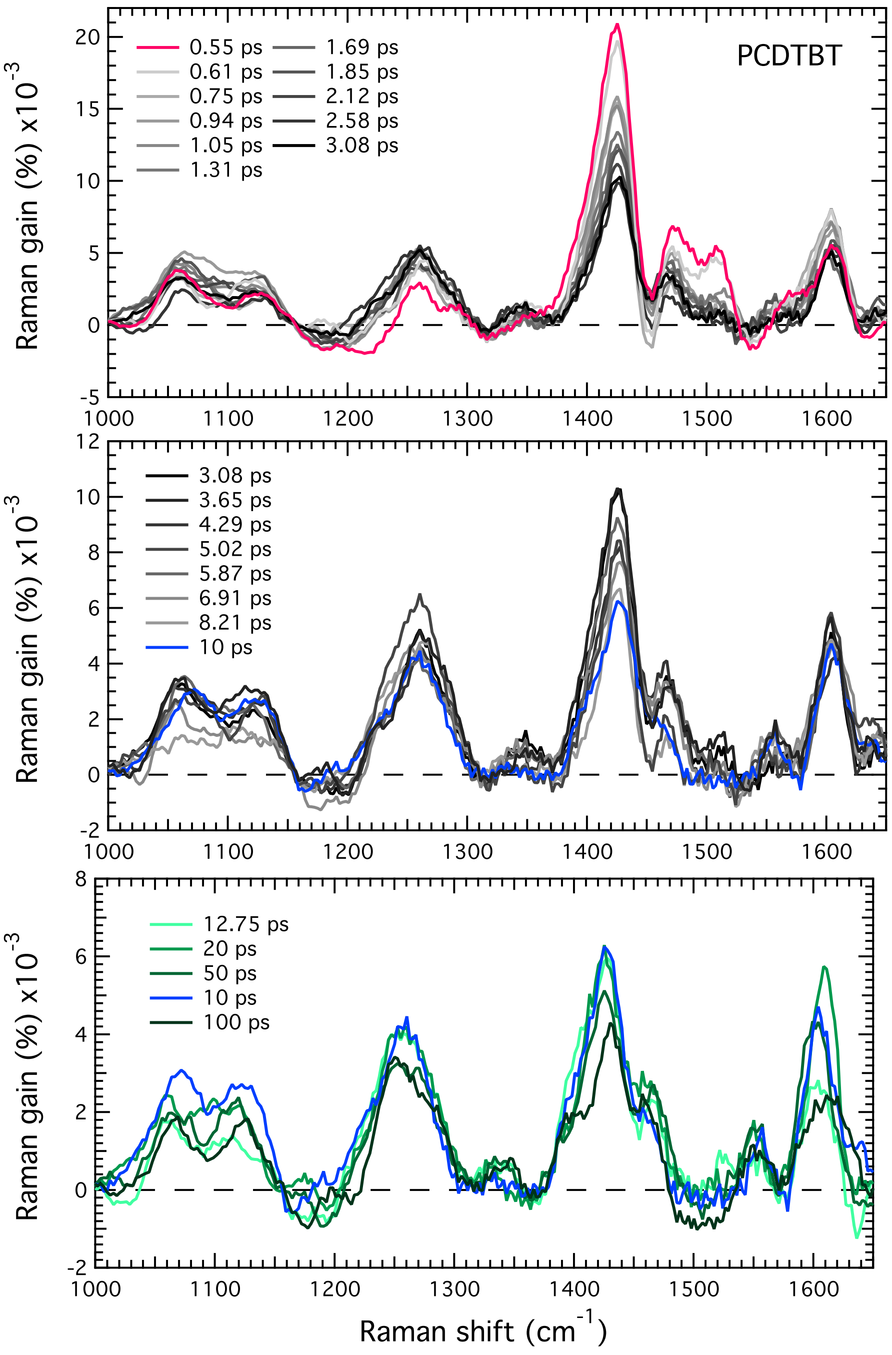


**Figure S8** Transient Raman spectra of PCDTBT film from 0.55 ps to 100 ps, divided in 3 panels to better illustrate the spectral evolution.

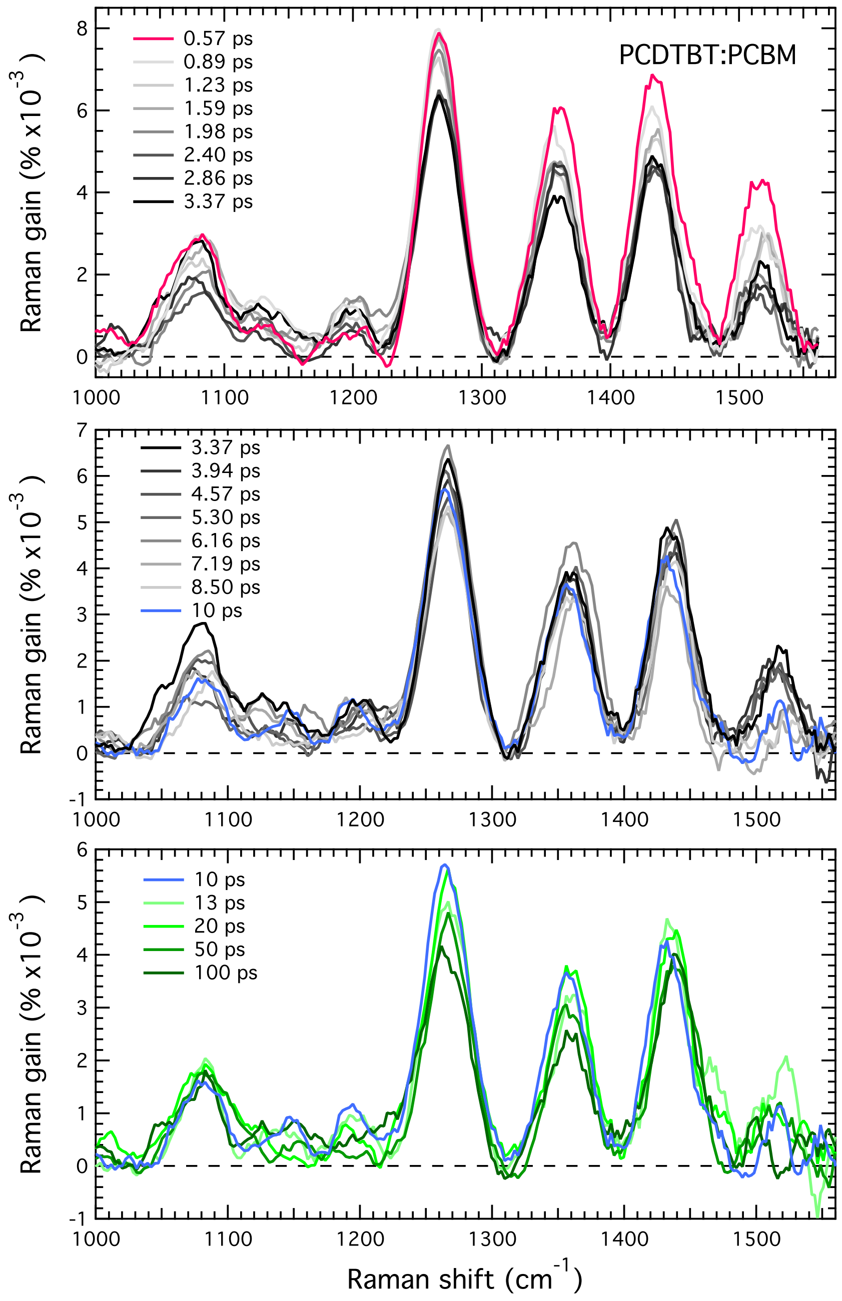


**Figure S9** : Transient Raman spectra of PCDTBT:PCBM film from 0.57 ps to 100 ps, divided in 3 panels to better illustrate the spectral evolution.

**Molecular orbitals of the PCDTBT cation**

The molecular orbitals of the cation differ from the neutral PCDTBT. In first approximation, since an electron is missing in the HOMO of the (formally neutral) polymer, the latter becomes the LUMO of the cationic PCDTBT. Similarly, the HOMO-1 of neat PCDTBT becomes the HOMO of cationic PCDTBT.

However, the cation breaks the spin symmetry of neutral PCDTBT because of the missing electron, which affects the HOMO of the cation. It is a mix of the HOMO and HOMO-1 of the neutral PCDTBT, and the HOMO of the cation sits 130 meV above the HOMO of neat PCDTBT.

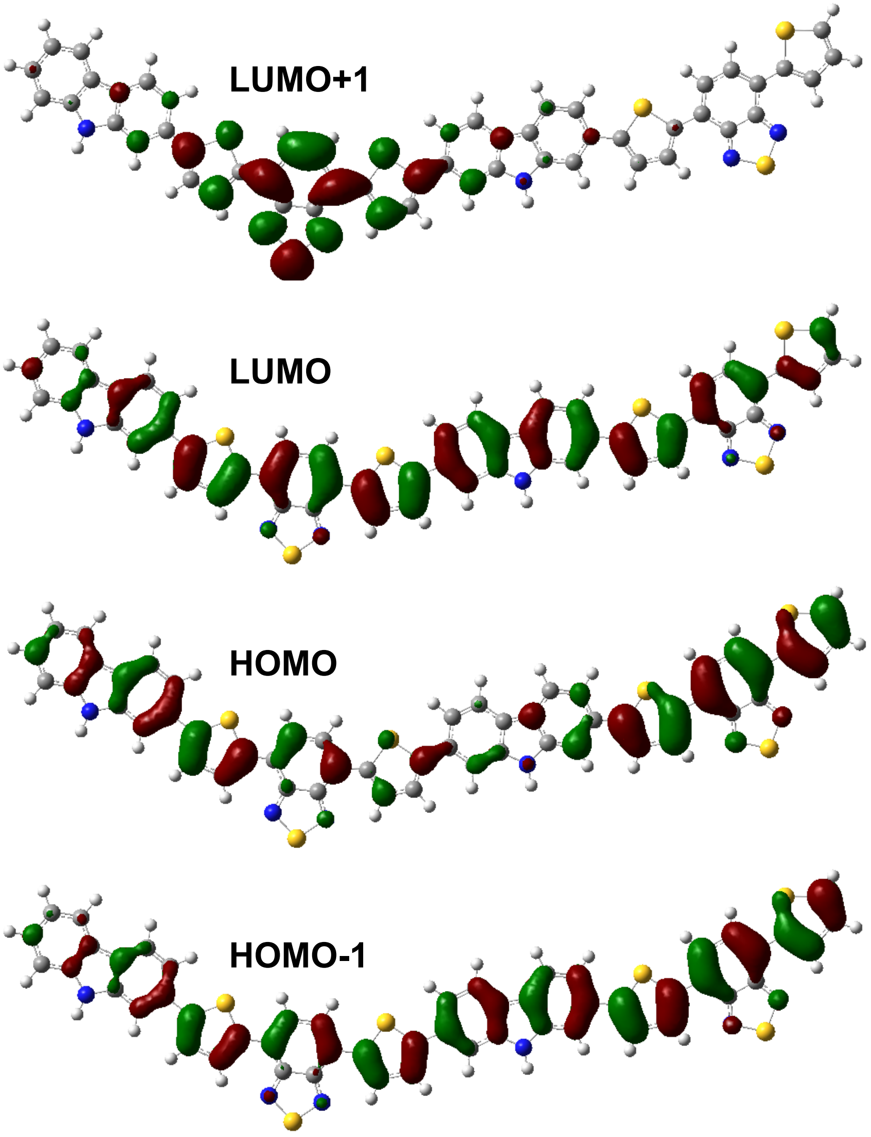


**Figure S10 :** Molecular orbitals of the PCDTBT cation, from top to bottom.

## Important Raman modes

In the blend film, the fast disappearing peak around 1513 $cm^{-1}$ is a carbazole mode coupled to thiophenes. This mode is present in the resonance Raman of doped PCDTBT and have a calculated frequency of 1540 $cm^{-1}$ :

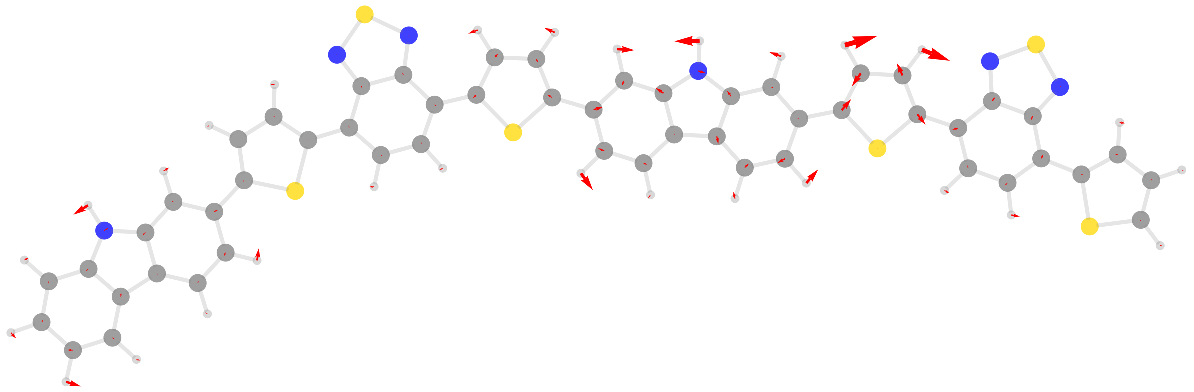

The same carbazole mode exists in the neat PCDTBT, but since the electronic density is different, it couples to the thiophenes to a lesser extent, resulting in almost no Raman activity / intensity. This mode has a calculated frequency of 1543 $cm^{-1}$ :

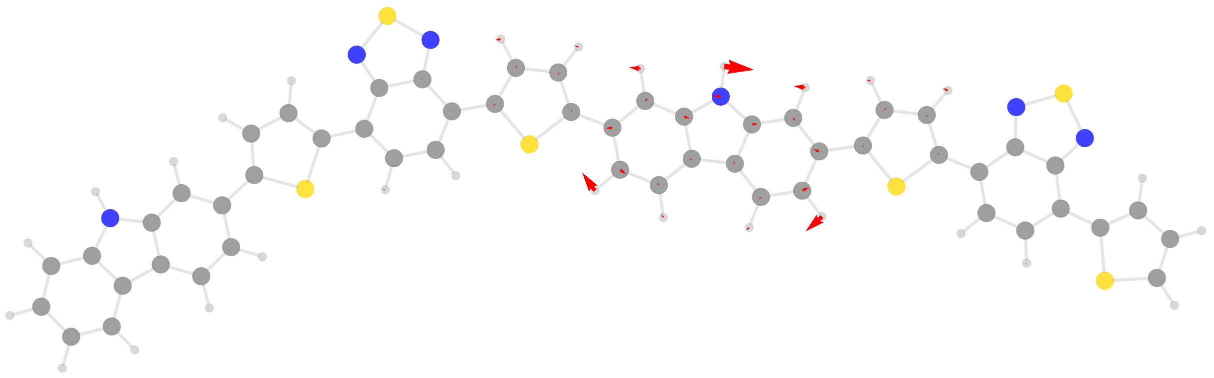

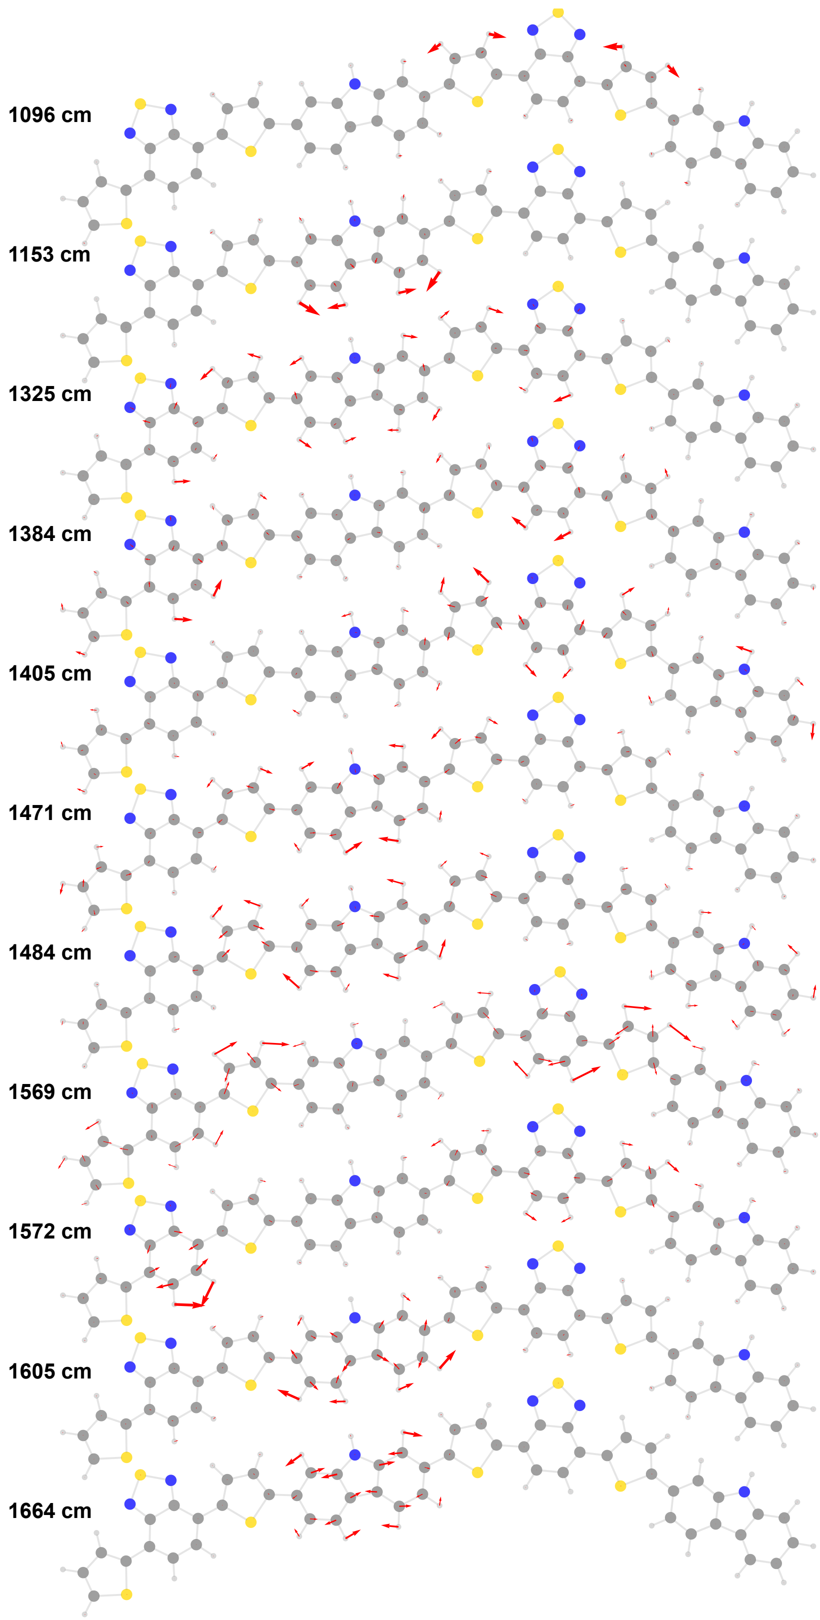


**Figure S11 :** Neutral PCDTBT calculated vibrational modes

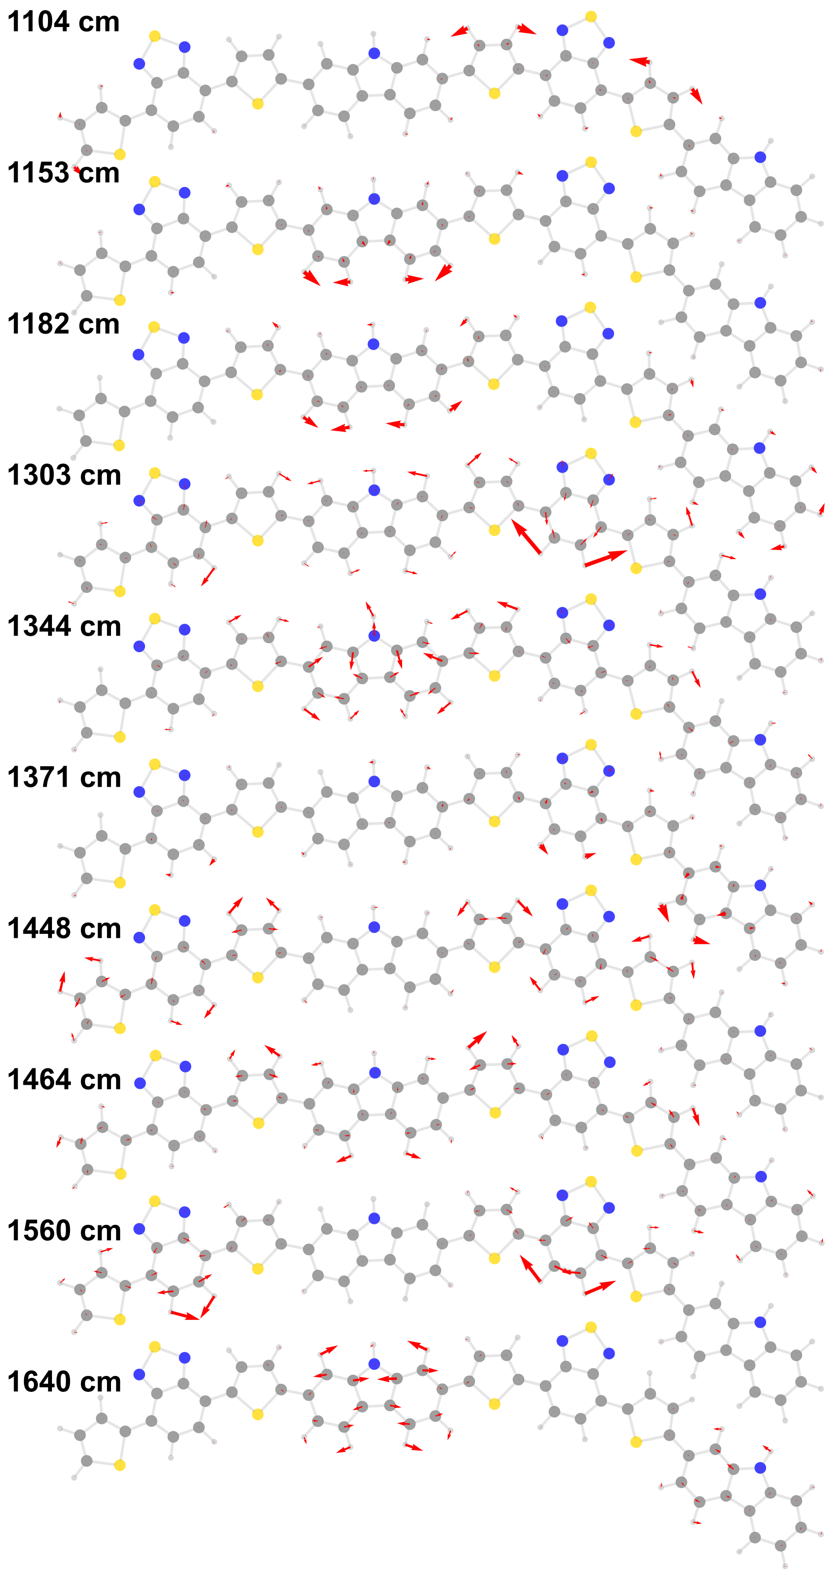


**Figure S12 :** Cationic PCDTBT calculated vibrational modes

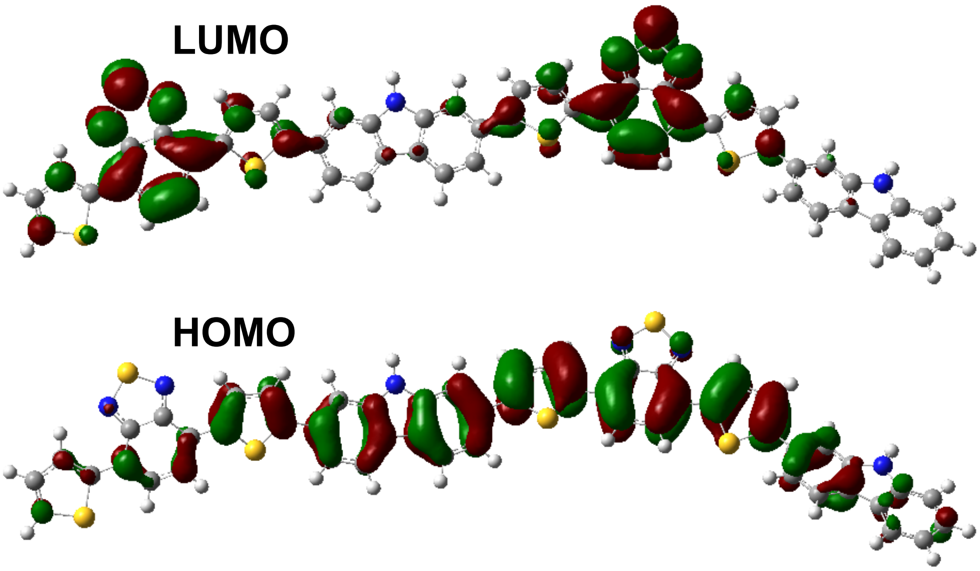


**Figure S13 :** Neutral PCDTBT frontier orbitals. Note the shift of the electron density from the carbazole to the benzothiodiazole moiety, lengthening thus the carbazole C-C bonds.

## References

1. Blouin, N. *et al.* Toward a rational design of poly (2, 7-carbazole) derivatives for solar cells. *J. Am. Chem. Soc.* **130,** 732–742 (2008).
2. Park, S. *et al.* Bulk heterojunction solar cells with internal quantum efficiency approaching 100%. *Nature Photonics* **3,** 297–302 (2009).
3. Rispens, M. T. *et al.* Influence of the solvent on the crystal structure of PCBM and the efficiency of MDMO-PPV:PCBM 'plastic' solar cells. *Chem. Commun.* 2116–2118 (2003). doi:10.1039/B305988J
4. Verploegen, E. *et al.* Effects of Thermal Annealing Upon the Morphology of Polymer-Fullerene Blends. *Advanced Functional Materials* **20,** 3519–3529 (2010).
5. Westacott, P. *et al.* On the role of intermixed phases in organic photovoltaic blends. *Energy Environ. Sci.* **6,** 2756–2764 (2013).
6. Collins, B. A. *et al.* Molecular Miscibility of Polymer−Fullerene Blends. *J. Phys. Chem. Lett.* **1,** 3160–3166 (2010).
7. Watts, B., Belcher, W. J., Thomsen, L., Ade, H. & Dastoor, P. C. A Quantitative Study of PCBM Diffusion during Annealing of P3HT:PCBM Blend Films. *Macromolecules* **42,** 8392–8397 (2009).
