# Supplementary material for: Direct observation of ultrafast long-range charge separation at polymer:fullerene heterojunctions
Source: arXiv:1310.8331 ancillary file (2013-10-30)
Supplement: Supplementary file 2 [file FSRS_paper_figures-V5.pdf]

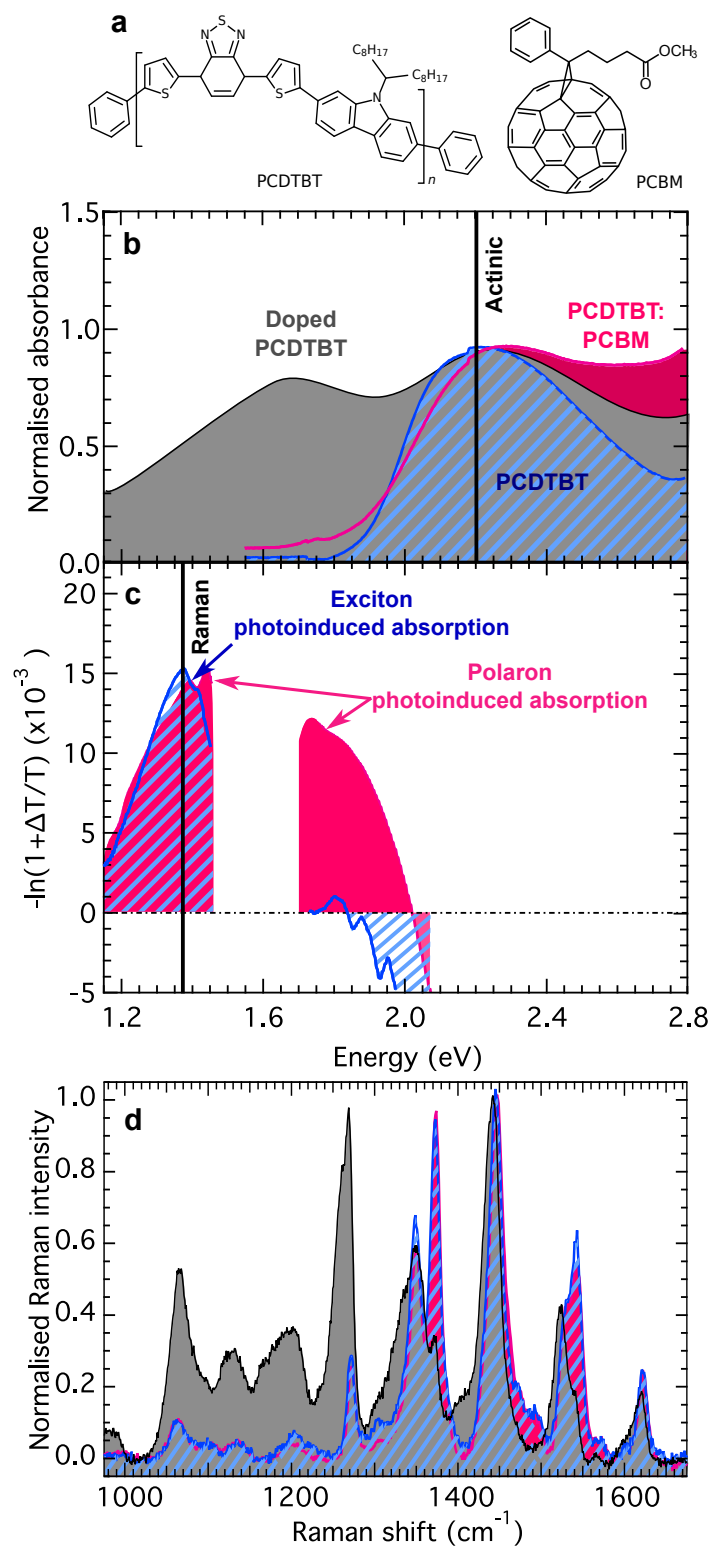

Provencher Fig. 1

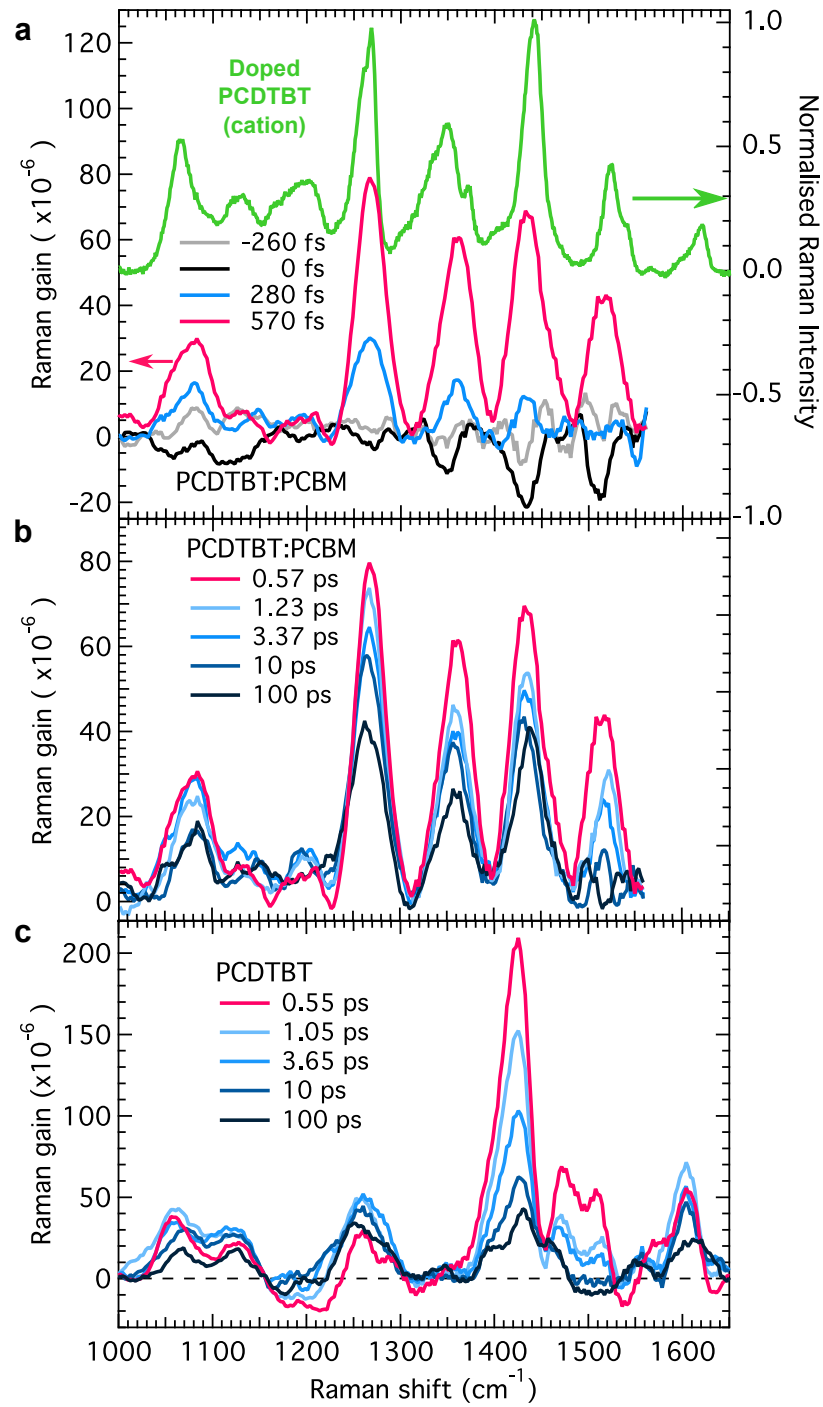

Provencher Fig. 2

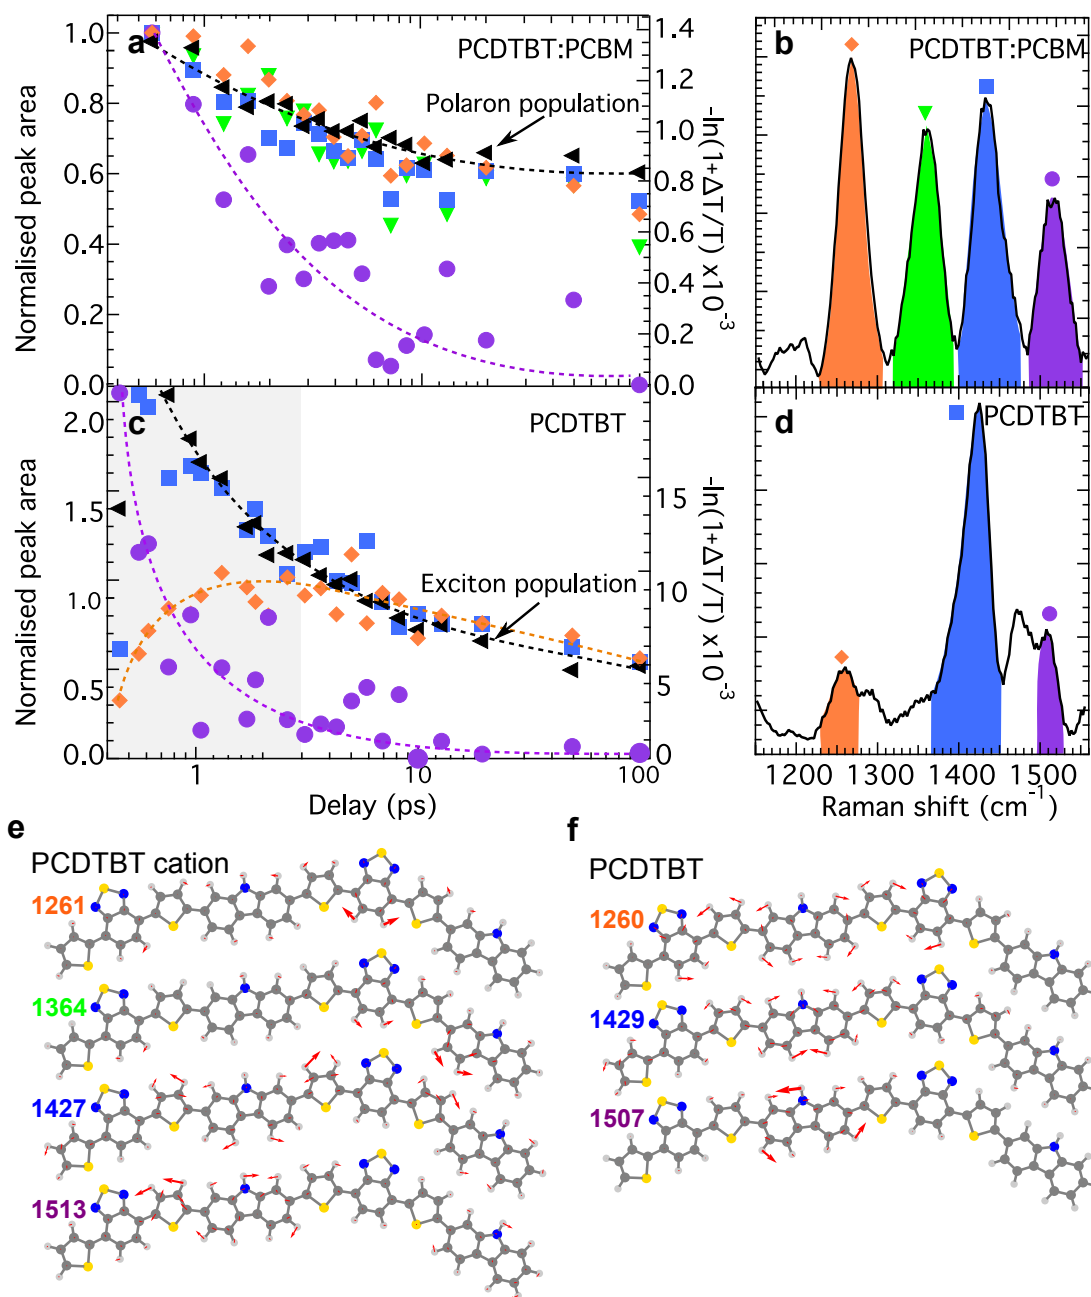

Provencher Fig. 3
